# Supplementary material for: Hybrid Audio Detection Using Fine-Tuned Audio Spectrogram Transformers: A Dataset-Driven Evaluation of Mixed AI-Human Speech
Source: arXiv:2505.15136 source file (2025-05-21)
Supplement: Supplementary file 1 [file appendix.tex]

\newpage
\appendix
\setcounter{table}{0}
\section{Appendix}
\label{sec:appendix}
\subsection{Additional Experimental Results}
\label{subsec:Results}
\subsubsection{LeNet300-100 on MNIST}
\label{subsubsec:letnet300}
We conduct experiments with LeNet-300-100 using the same parameters and settings on the MNIST dataset. 
Table~\ref{table:lenet300_mnist} compares the results with existing filter pruning methods and weight pruning methods. The results show that MIXP can achieve high weight CR of $97.5\%$ without loss of accuracy using only $4k$ retraining iterations. It is obvious that MIXP has a low Re-Iters of $4k$ with a comparably high weight CR of $98.3\%$ and $\Delta Acc$ of $-0.3$. We note that although L-OBS* exhibits the fewest Re-Iters in the table, it suffers from much more computational cost in each pruning iteration than MIXP (i.e., $O(J^3)$ (L-OBS*) v.s. $O(J^2)$ (MIXP)). The experimental results demonstrate our MIXP approach can be applied to the fully connected neural network with high weight CR.
\begin{table}[!htbp]
	\centering
	\small
	\begin{tabular}
		{m{2cm}<{\centering} m{1.6cm}<{\centering}  m{1.6cm}<{\centering} m{1.4cm}<{\centering}}
		\Xhline{2\arrayrulewidth}
		%  \multicolumn{4}{c}{Filter Pruning Methods}\\
		
		%  \multicolumn{4}{c}{Weight Pruning Methods}\\
		Weight Pruning Method &\begin{tabular}{@{}c@{}}Weight CR($\%$)\end{tabular} & \(\Delta\)Acc($\%$)  & Re-Iters \\  % inserts table %heading
		\hline
		SWS  & 95.6 & -0.2 & - \\
		GDF  & 95.8 & 0.0 & -\\
		LC  & 99.0 & -1.5 & - \\
		LWC & 92.3 & 0.0 & 96K \\
		OBD& 92.0 & -0.3 & 81K \\
		GSM  & 98.3 & 0.0 & 61K \\
		DNS & 98.2 & -0.3 & 34K \\
		SNIP  & 98.0 & -0.7 & 25K \\
		FDNP  & 99.2 & 0.0 & 20K \\
		\textbf{Ours} & \textbf{97.5 / 98.3} & \textbf{0.0 / -0.3} & \textbf{4k}\\
		L-OBS*  & 98.5 & -0.3 & 510 \\
		\Xhline{2\arrayrulewidth}
	\end{tabular}
	\caption{Comparison of different weight pruning methods for compressing LeNet-300-100 on the MNIST dataset. For reference, in our implementation, the accuracy of the uncompressed model is $98.2\%$. }
	%The L-OBS* exhibits the fewest re-train iterations but suffers from much more pruning iterations. }
	\label{table:lenet300_mnist}
\end{table}
\subsubsection{MobileNet on on CIFAR-10}
We also conduct experiments with MobileNet-V1 and MobileNet-V2 on the CIFAR-10 dataset. 
%Instead of using standard convolutions, MobileNet-V1 are based on a form of factorized convolutions called depthwise separable convolution. 
%Depthwise separable convolutions consist of a depthwise convolution followed by a 1x1 convolution called a pointwise convolution. 
%This factorization significantly reduces the number of parameters in the model by filtering and combining input channels in two separate steps instead of together as in the standard convolution. 
%The MobileNet-V1 architecture consists of one standard convolution layer acting on the input image, a stack of depthwise separable convolutions, and finally averaging pooling and fully connected layers. 
%The MobileNet-V2 architecture is based on an inverted residual structure where the input and output of the residual block are thin bottleneck layers opposite to traditional residual models which use expanded representations in the input. MobileNetV2 provides a very efficient mobile-oriented model. 
%MobileNet-V2 aims to provide a more efficient mobile-oriented model by introducing an inverted residual structure and removing Non-linearities in narrow layers.
%A width multiplier is used in MobileNet -V1 and -V2 to the trade-off between the accuracy and the number of parameters. 
%In addition, both MobileNet -V1 and -V2 use a width multiplier that allows trading off the accuracy of the model with the number of parameters and computational cost.
A width multiplier is used in MobileNet -V1 and -V2 to the trade-off between the accuracy and the number of parameters. The range of the width multiplier is $(0, 1]$. The width multiplier of the baseline model is 1.0, which means baseline models keeps the original number of input and output channels in each layer. The number of input channels and output channels in each layer is scaled by setting the width multiplier between $(0, 1)$. 
%For a given width multiplier i $\in (0, 1]$ , the number of input channels and output channels in each layer is scaled by width multiplier relative to the 1.0 baseline model. 
We compare the accuracy performance of baseline MobileNets trained with width multipliers 1,  0.75, 0.5, and 0.25 with the performance of pruned MobileNets pruned from 1.0 baseline MobileNet and DCP in Table~\ref{table:mobilenet_filter} on the CIFAR-10 dataset. We see that pruned MobileNets are able to outperform baseline MobileNets. Specifically, Our MIXP has $20\%$ and 30$\%$ higher weight CR and FLOPs CR than the $0.5$ baseline MobileNet-V1, respectively. Similarly, it can achieve $23\%$ and $22\%$ higher weight CR and FLOPs CR than the $0.75$ baseline MobileNet-V2, respectively.  
MIXP also outperforms DCP in weight and FLOPs CR. Our MIXP has $53\%$ and 23$\%$ higher weight CR and FLOPs CR than the DCP on MobileNet-V1 and $21\%$ and 36 $\%$ higher weight CR and FLOPs CR than the DCP on MobileNet-V2, respectively. Note that MIXP can improve the accuracy of MobileNet-V1 and -V2 by $0.3\%$ and $0.15$ as DCP does. The results demonstrate that MIXP can effectively reduce computational cost and weight size of complex models for complex datasets.
\begin{table}[!htbp]	
	\centering
	\small
	\begin{tabular}
		{m{0.1cm}<{\centering} m{2.1cm}<{\centering} m{1.0cm}<{\centering}  m{1.0cm}<{\centering}  m{1.4cm}<{\centering}}
		\Xhline{2\arrayrulewidth}
		\quad & Method &\begin{tabular}{@{}c@{}}Weight \\CR($\%$)\end{tabular} & \begin{tabular}{@{}c@{}}FLOPs \\CR($\%$)\end{tabular} & \(\Delta\)Acc($\%$) \\  % inserts table %heading		
		\hline
		\multirow{6}*{\rotatebox{90}{Mobilenet-V1}}
		&1$\times$ baseline &0.0&0.0& 0.0 \\
		~&0.75$\times$ baseline &43.0  &43.5 & -0.7 \\
		~&0.50$\times$ baseline &74.9 &74.7& -1.2 \\
		~&0.25$\times$ baseline  & 93.8&93.6& -5.8 \\
		~&DCP  &58.0&73.8& +0.41 \\
		~&\textbf{MIXP (Ours)} &\textbf{ 89.2} & \textbf{90.2} & \textbf{+0.3} \\ 
		\hhline{=====}
		\multirow{6}*{\rotatebox{90}{Mobilenet-V2}}
		\\
		&1$\times$ baseline &0.0&0.0& 0.0 \\
		~&0.75$\times$ baseline &41.0  &45.1 & -0.9 \\
		~&0.50$\times$ baseline &78.9 &73.1& -1.8 \\
		~&DCP  &56.0&57& +0.22 \\
		~&\textbf{MIXP (Ours)} &\textbf{ 68.6} & \textbf{78.9} & \textbf{+0.15} \\ 
		\Xhline{2\arrayrulewidth}
	\end{tabular}
	\caption{Comparison of different filter pruning methods for compressing MobileNet-V1 and -V2 on the CIFAR-10 dataset. For reference, in our implementation, the accuracy of the uncompressed MobileNet-V1 model is $93.1\%$, MobileNet-V2 model is $92.8\%$.}
	\label{table:mobilenet_filter}
\end{table}
\subsubsection{Additional Ablation Evaluation}
\begin{table}[!htbp]
	\centering
	\small
	\begin{tabular}
		{m{3.0cm}<{\centering} m{1.4cm}<{\centering} m{1.4cm}<{\centering}  m{1.4cm}<{\centering} }
		\Xhline{2\arrayrulewidth}
		\quad  & Connection CR(\%) & Weight CR(\%)  & FLOPs CR(\%)
		\\ % inserts table %heading		
		\hline
		
		\begin{tabular}{@{}c@{}}MIXP\\(connection pruning only)\end{tabular} &90  & 86 & 65  \\
		\begin{tabular}{@{}c@{}}MIXP\\(weight pruning only)\end{tabular}&-  & 98 & 89 \\
		\begin{tabular}{@{}c@{}}\textbf{MIXP}\end{tabular}&90  &98 & \textbf{97}  \\
		\Xhline{2\arrayrulewidth}
	\end{tabular}
	\caption{Performance with different pruning components in MIXP on Lenet-5.}
	\label{table:ablation}
\end{table}
We conduct the experiments to present the effects of different pruning components on the overall performance. As shown in Table~\ref{table:ablation}, when the pruned model achieves 90\% connection CR only using connection pruning in MIXP, it has 86\% weight CR and 65\% FLOPs reduction. However, under the same achieved connection CR, our full method, MIXP, has 98\% weight CR and 97\% FLOPs reduction. This result demonstrates that adopting weight pruning after the connection pruning could indeed achieve a better compression ratio and lower FLOPs. Moreover, when only using the weight pruning in MIXP, it achieves 89\% FLOPs reduction which is 8\% lower than full MIXP under the same achieved weight CR 98\%. This result shows that the connection pruning could help reduce the FLOPs than using weight pruning alone.
Overall, both connection and weight pruning of our approach play a significant role in improving the performance of MIXP.
